# Supplementary material for: MEND: RL For Flow Models via Proximal Velocity Matching
Source: arXiv:2610.05954 source file (2026-10-05)
Supplement: Supplementary file 1 [file v2_A_notation.tex]

\section{Algorithm as implemented}\label{app:notation}\label{app:design}\label{app:alg}
Algorithm~\ref{alg:impl} is Algorithm~\ref{alg:mend} with the bookkeeping of the implementation: the global cap floor, the tie rules, the price controller and the two EMAs. Notation follows Section~\ref{sec:method}; $Q_q$ is the $q$-quantile of a set, $u$ the update index and $a$ the acceptance share. Rewards, cap statistics and loss normalizers are pooled over devices.
\begin{algorithm}[!h]
\caption{\mend{}: one training round, as implemented.}\label{alg:impl}
\small
\begin{algorithmic}[1]
\Require adapters $\theta$, $\theta_{\mathrm{old}}$, $\theta_{\mathrm{ema}}$; price $\tau$; floor $\kappa_{\mathrm{glob}}$; update index $u$
\State Roll out $\theta_{\mathrm{old}}$ for every prompt $c$ and seed; store the endpoint $x$ and the state $z_q$ \Comment{rollout}
\State $R(x,c)$ and $g=\nabla_x R(x,c)$ for every sample, in one backward pass \Comment{score}
\State Raise $\kappa_{\mathrm{glob}}$ toward the round's median reward; never lower it \Comment{floor}
\State $\kappa(c)\gets\max\{Q_q(\{R(x^{(k)},c)\}_{k}),\ \kappa_{\mathrm{glob}}\}$ for every prompt \Comment{cap}
\For{each sample with $R(x,c)<\kappa(c)$}
  \State $y_j\gets x+\eta_j\,g/\norm{g}$ for $j=1,\ldots,K$ \Comment{propose}
  \State $\ystar\gets\arg\max_{y\in\{x,y_1,\ldots,y_K\}}\Rk(y,c)-\norm{y-x}^2/(2\tau)$; ties to $x$, then to the shortest \Comment{verify}
\EndFor
\State $d\gets\ystar-x$ for moved samples; $d\gets 0$ for every other sample
\State One AdamW step on $\mathcal L(\theta)$ of \eqref{eq:loss}; $u\gets u+1$ \Comment{regress}
\State $\theta_{\mathrm{ema}}\gets\nu_u\theta_{\mathrm{ema}}+(1-\nu_u)\theta$ \Comment{evaluated weights}
\State $a\gets$ share of proposed samples that moved; rescale $\tau$ if $a$ leaves its band; clamp \Comment{price}
\State $\theta_{\mathrm{old}}\gets\mu_u\theta_{\mathrm{old}}+(1-\mu_u)\theta$ \Comment{behavior}
\end{algorithmic}
\end{algorithm}
