# Supplementary material for: MEND: RL For Flow Models via Proximal Velocity Matching
Source: arXiv:2610.05954 source file (2026-10-05)
Supplement: Supplementary file 2 [file v2_B_settings.tex]

\section{Evaluation settings}\label{app:settings}\label{app:cfg}\label{app:extra}
\paragraph{Protocols.} Protocol~O follows \citet[Appendix~C.1]{zhou2026opsd}: SD3.5-M with a LoRA adapter, $\hpPromptsO\times\hpImagesO$ Pick-a-Pic images per update for \hpUpdatesO{} updates, and evaluation on DrawBench $200\times5$ at guidance 1. The development budget uses $16\times8$ images per update for 50 updates and is scored on DrawBench prompts 1 to 64 with two seeds. Every \mend{} run trains without guidance except Protocol~F, which trains and samples at 4.5. The settings behind each main-text figure and table are:
\begin{itemize}[leftmargin=1.4em, itemsep=1pt, topsep=2pt]
\item Figure~\ref{fig:hero}(a) to (c), Figure~\ref{fig:rewards}, Table~\ref{tab:transfer} and Section~\ref{sec:frontier}: Protocol~O, guidance 1, update 100, no checkpoint selection. Panel (a) is the training reward as a trailing mean over five updates.
\item Table~\ref{tab:main}: \mend{} at guidance 4.5 and update 100; the base and the Flow-GRPO adapter at 4.5; the DiffusionNFT checkpoint at 1. The three-reward row (PickScore$/26$ + CLIPScore + HPSv2.1) is sampled at guidance 1 at update 300.
\item Figure~\ref{fig:dynamics}: panel (a) at guidance 1 on val64, panels (b) and (c) at 4.5; the Flow-GRPO and DiffusionNFT levels at their own settings.
\item Tables~\ref{tab:sd3m} and~\ref{tab:zimage}: guidance 1, update 100; Z-Image-Turbo uses 9 Euler steps at 1024 pixels.
\item Figure~\ref{fig:ablation} and Table~\ref{tab:ablation}: development budget, guidance 1, update 50. Table~\ref{tab:sensitivity}: Protocol~O budget, guidance 1, update 50, DrawBench prompts 65 to 200 with two seeds.
\item Images: Figures~\ref{fig:cmp}, \ref{fig:qual} and~\ref{fig:cmp2} and columns 1, 4 and 5 of Figure~\ref{fig:hero} are 1024-pixel renders at each model's headline setting; Figures~\ref{fig:fidelity} and~\ref{fig:progress} and columns 2 and 3 of Figure~\ref{fig:hero} are 512-pixel renders at guidance 4.5. Figure~\ref{fig:method} is logged at update 25 from the rollout policy.
\item Appendix figures: in Figure~\ref{fig:perreward}, thick curves sample \mend{} at 4.5 and light curves at 1; ReFL and DiffusionNFT curves use 1.
\end{itemize}

\subsection{Baselines}\label{app:baselines}
ReFL and DiffusionNFT under Protocol~O, the rows marked $^\dagger$ and the corresponding curves, follow \citet{zhou2026opsd}. Flow-GRPO is the PickScore adapter of \citet{liu2025flowgrpo}, trained for about 4k updates with a KL penalty at guidance 4.5. DiffusionNFT outside Protocol~O is the five-reward checkpoint of \citet{zheng2025nft}, trained for 1.7k iterations. Both are evaluated at their own settings in the pipeline of Appendix~\ref{app:evalproto}, from the same initial noise as \mend{}. Neither matches Protocol~O, so the $^\dagger$ rows are the matched comparison.

The pipeline agrees with the original papers: SD3.5-M gives PickScore 20.58 against 20.51 at guidance 1 and 22.35 against 22.34 at 4.5, the Flow-GRPO adapter 23.52 against 23.53, and the DiffusionNFT checkpoint 23.82 against 23.80. The DiffusionNFT curves of Figures~\ref{fig:dynamics}(a), \ref{fig:frontier-main} and~\ref{fig:frontier-div} and the open triangles of Figure~\ref{fig:perreward} come from a Protocol~O run in this pipeline, which reaches 23.45 against 23.43 in \citet{zhou2026opsd}.

\subsection{Evaluation protocol}\label{app:evalproto}
DrawBench \citep{saharia2022imagen}, $\hpEvalPrompts\times\hpEvalSeeds$ images, 40-step Euler flow ODE, \hpRes{} pixels, EMA weights for \mend{}. The initial noise of each (prompt, seed) pair is shared across methods, and intervals are 95\% prompt-bootstrap intervals. Diversity is the mean pairwise DreamSim \citep{fu2023dreamsim} cosine distance among a prompt's images, averaged over prompts; distance to the base is the DreamSim distance to the base image from the same noise and guidance.

For an image with luma $Y\in[0,1]$, let $E_{\mathrm{hf}}$ be the power of the Hann-windowed 2D FFT of $Y - \bar Y$ in the band $0.08 \le |f| < 0.25$ cycles per pixel. The HF ratio of a method is $\exp\big(\E_p \E_s \log E_{\mathrm{hf}}(\text{method})/E_{\mathrm{hf}}(\text{ref})\big)$ over prompts $p$ and seeds $s$, with SD3.5-M at guidance \hpRefCFG{} as reference.

\begin{figure}[!t]
\centering
\includegraphics[width=\linewidth]{figures/v2_appx/fig_cfg_sweep.pdf}
\caption{\textbf{Guidance trades reward components against diversity.} Val64 ($64\times2$, 512 pixels) for the baselines and \mend{} at update 100; the marked setting is guidance 4.5.}
\label{fig:cfg-sweep}
\end{figure}

\subsection{Guidance}\label{app:campaign-protf}\label{app:guidance-images}\label{app:ext-protf}
Figure~\ref{fig:cfg-sweep} sweeps guidance on val64, 64 Pick-a-Pic prompts disjoint from DrawBench. \mend{}'s PickScore is highest at guidance 1 and falls slowly, while guidance raises HPSv2.1, ImageReward and CLIPScore and lowers diversity for every model. Protocol~F trains \mend{} at guidance 4.5 for 100 updates without a KL term (Table~\ref{tab:protf}).
\begin{table}[!htbp]
\centering
\caption{\textbf{Training with guidance.} Protocol~F and the Flow-GRPO PickScore adapter, DrawBench $200\times5$; both train and sample at guidance 4.5, with different budgets and regularizers.}
\label{tab:protf}
\small\setlength{\tabcolsep}{3pt}
\resizebox{\linewidth}{!}{%
\begin{tabular}{lccccccccccc}
\toprule
Method & Upd. & Setting & Reg. & PickScore & HPSv2.1 & HPSv3 & ImageReward & CLIPScore & Aesthetic & Div. & Dist. \\
\midrule
Flow-GRPO, PickScore adapter & ${\sim}$4k & 4.5/4.5 & KL & 23.52 & 0.316 & 7.04 & 1.27 & 0.280 & 5.90 & 0.202 & 0.313 \\
\oursrow \mend{}, trained with guidance (Protocol~F) & 100 & 4.5/4.5 & none & \res{pf.pick} & \res{pf.hps2} & \res{pf.hps3} & \res{pf.ir} & \res{pf.clip} & \res{pf.aes} & \res{pf.div} & \res{pf.dist} \\
\bottomrule
\end{tabular}}
\end{table}
\begin{figure}[!htbp]
\centering
\begin{minipage}[t]{0.49\linewidth}
\centering
\noindent\parbox[b]{0.2500\linewidth}{\centering\scriptsize CFG 1}\parbox[b]{0.2500\linewidth}{\centering\scriptsize CFG 2}\parbox[b]{0.2500\linewidth}{\centering\scriptsize CFG 3}\parbox[b]{0.2500\linewidth}{\centering\scriptsize CFG 4.5}\\[1pt]
\includegraphics[width=\linewidth]{figures/qual/qual_cfg_matrix_a_row0.jpg}\\[-1pt]
{\scriptsize SD3.5-M. Seed 43: close up photo of a rabbit, forest, haze, halation, bloom, dramatic atmosphere, centred, rule of thirds, 200mm 1.4f macro shot}\\[3pt]
\includegraphics[width=\linewidth]{figures/qual/qual_cfg_matrix_a_row1.jpg}\\[-1pt]
{\scriptsize Flow-GRPO}\\[3pt]
\includegraphics[width=\linewidth]{figures/qual/qual_cfg_matrix_a_row2.jpg}\\[-1pt]
{\scriptsize DiffusionNFT}\\[3pt]
\includegraphics[width=\linewidth]{figures/qual/qual_cfg_matrix_a_row3.jpg}\\[-1pt]
{\scriptsize \mend{}, update 100}\\[3pt]

\end{minipage}\hfill
\begin{minipage}[t]{0.49\linewidth}
\centering
\noindent\parbox[b]{0.2500\linewidth}{\centering\scriptsize CFG 1}\parbox[b]{0.2500\linewidth}{\centering\scriptsize CFG 2}\parbox[b]{0.2500\linewidth}{\centering\scriptsize CFG 3}\parbox[b]{0.2500\linewidth}{\centering\scriptsize CFG 4.5}\\[1pt]
\includegraphics[width=\linewidth]{figures/qual/qual_cfg_matrix_b_row0.jpg}\\[-1pt]
{\scriptsize SD3.5-M. Seed 43: 38 year old man, black hair, black stubble, colombian, immense detail/ hyper. Pårealistic, city /cyberpunk, high detail, detailed, 3d, trending on artstation, cinematic}\\[3pt]
\includegraphics[width=\linewidth]{figures/qual/qual_cfg_matrix_b_row1.jpg}\\[-1pt]
{\scriptsize Flow-GRPO}\\[3pt]
\includegraphics[width=\linewidth]{figures/qual/qual_cfg_matrix_b_row2.jpg}\\[-1pt]
{\scriptsize DiffusionNFT}\\[3pt]
\includegraphics[width=\linewidth]{figures/qual/qual_cfg_matrix_b_row3.jpg}\\[-1pt]
{\scriptsize \mend{}, update 100}\\[3pt]

\end{minipage}
\caption{\textbf{Guidance sweep in images.} Guidance 1, 2, 3 and 4.5 (columns) for SD3.5-M, Flow-GRPO, DiffusionNFT and \mend{} at update 100 (rows); two val64 prompts, seed 43, 512 pixels, selected by eye. DiffusionNFT over-saturates as guidance grows.}
\label{fig:qual-cfg-matrix}
\end{figure}

\subsection{Other held-out checks}\label{app:heldout-checks}\label{app:geneval}\label{app:geneval-qual}
GenEval \citep{ghosh2023geneval} and Flow-GRPO's OCR benchmark are run with the scripts of \citet{liu2025flowgrpo}; no \mend{} run trains on either. At guidance 1 \mend{} scores \res{gmend.overall} on GenEval against \res{gbase1.overall} for its base; at guidance 4.5 it matches the Flow-GRPO PickScore adapter on GenEval (\res{gmend45.overall} against \res{gfgpick.overall}) and is below it on OCR (\res{omend45.ocr} against \res{ofgpick.ocr}). Figures~\ref{fig:frontier-main} and~\ref{fig:frontier-div} place \mend{} and DiffusionNFT under Protocol~O on the reward-distance and reward-diversity planes along training.
\begin{figure}[!htbp]
\centering
\input{figures/snippets/v2_fig_frontier_a}\hfill
\input{figures/snippets/v2_fig_frontier_b}
\end{figure}
