# Supplementary material for: MEND: RL For Flow Models via Proximal Velocity Matching
Source: arXiv:2610.05954 source file (2026-10-05)
Supplement: Supplementary file 3 [file v2_C_proofs.tex]

\section{Theory: statements and proofs}\label{app:proofs}
\newcommand{\mendrestatename}{Theorem}
\theoremstyle{plain}
\newtheorem*{mendrestate}{\mendrestatename}
\theoremstyle{remark}
This appendix proves the results of Section~\ref{sec:theory}. The guarantees concern target selection and first-order prediction changes, not finite optimizer steps or full training runs (Remark~\ref{rem:notprox}).

\paragraph{Conventions.} All quantities refer to one round. Latents lie in $\R^D$ with inner product $\ip{u}{w}=D^{-1}\sum_{j=1}^D u_jw_j$ and RMS norm $\norm{u}=\ip{u}{u}^{1/2}$. All latent distances use this norm, with $\mathrm{dist}(x,\emptyset)=+\infty$; $\Wtwo^2$ denotes the infimum of expected squared distance over couplings. We suppress the prompt and write $R(x)=R_{\mathrm{img}}(\mathrm{Dec}(x),c)$. Its gradient for this inner product is $D$ times the Euclidean gradient. RMS normalization cancels this factor, so the implementation and analysis give the same direction $\hat h=g/\norm{g}$ for $g\ne0$.

The behavior adapter rolls out $n$ seeds to endpoints $x_i$ and stored states $z_i$ near $t_q$. Let $g_i=\nabla R(x_i)$ and $\hat h_i=g_i/\norm{g_i}$ when $g_i\ne0$, with $\hat h_i=0$ otherwise. Index the positive proposal lengths so that $\eta_1\le\cdots\le\eta_K$. The accepted set is $\mathcal A$, and $d_i=\ystar_i-x_i=\eta_i\hat h_i$ for $i\in\mathcal A$, where $\eta_i$ is the selected length; otherwise $d_i=0$. With $\xhat_i^{\mathrm{old}}=\xhat_{\theta_{\mathrm{old}}}(z_i)$, \eqref{eq:loss} becomes
\[
\begin{gathered}
\mathcal L(\theta)=\sum_i w_i\norm{\xhat_\theta(z_i)-\sg[\xhat_i^{\mathrm{old}}+d_i]}^2,\\
w_i=\begin{cases}
1/|\mathcal A|, & i\in\mathcal A,\\
\lambda_{\mathrm{keep}}/(n-|\mathcal A|), & i\notin\mathcal A.
\end{cases}
\end{gathered}
\]
Empty subsets contribute no term, and $\lambda_{\mathrm{keep}}\ge0$.
Parameters lie in $\R^p$ with Euclidean inner product $\ip{\cdot}{\cdot}_\Theta$ and norm $\norm{\cdot}_\Theta$. Write $D_i(\theta)=\partial_\theta\xhat_\theta(z_i)$ and define its adjoint by $\ip{D_i(\theta)^*u}{\phi}_\Theta=\ip{u}{D_i(\theta)\phi}$. Thus $\nabla_\theta F(\xhat_\theta(z_i))=D_i(\theta)^*\nabla F(\xhat_\theta(z_i))$. Operator norms use these inner products, so $\norm{D_i^*}=\norm{D_i}$, and $u^\top Mv=\ip{u}{Mv}_\Theta$.

\paragraph{The implemented round.} Rollouts use $\theta_{\mathrm{old}}$, so $x_i$, $z_i$ and $g_i$ are fixed during regression. For samples below the cap with $g_i\ne0$, proposals are $y_{ij}=x_i+\eta_j\hat h_i$. The verdict maximizes $J_i(y)=\Rk(y)-\norm{y-x_i}^2/(2\tau)$ over the proposals and $x_i$. Ties favor $x_i$, then the shortest proposal. Zero-gradient seeds generate no proposals and are kept. Seeds at or above the cap are also kept: for any $y\ne x_i$, $J_i(y)<J_i(x_i)=\kappa_i$. After the update, $\theta_{\mathrm{old}}\leftarrow\mu_u\theta_{\mathrm{old}}+(1-\mu_u)\theta$. All statements use exact arithmetic.

\paragraph{Assumptions.} Each condition lists the results that require it.
\begin{enumerate}[label=(A\arabic*), leftmargin=2.6em, itemsep=1pt, topsep=2pt]
\item \textnormal{Frozen round} (all results). The behavior parameters, endpoints, stored states, gradients, caps, penalty scale $\tau>0$ and proposal lengths are fixed before regression and independent of $\theta$. Targets carry no gradient.
\item \textnormal{Verdict} (all results). Each finite candidate set contains the unchanged sample. Rewards are deterministic, moves require a strict improvement in $J_i$, and ties follow a fixed rule. Expressions containing $1/|\mathcal A|$ assume $\mathcal A\ne\emptyset$. If $\mathcal A=\emptyset$, $\mathcal L=P$, defined below; if $|\mathcal A|=n$, the keep term is absent.
\item \textnormal{Seeds} (Corollaries~\ref{cor:w2} and~\ref{thm:modes}). A random seed includes its prompt, initial noise and group, which determines its cap. With $\tau$ fixed, $\pi$ and $\pi'$ are the laws of $x$ and $\ystar$; for a finite round, they are empirical measures. Each gain uses the same seed-specific cap at both endpoints. The relevant maps are measurable, as holds for continuously differentiable rewards and the stated selection rule.
\item \textnormal{Smoothness} (Propositions~\ref{prop:firstorder} and~\ref{prop:transfer}, Remark~\ref{rem:draft}). Rewards are differentiable at rollout endpoints, and $\theta\mapsto\xhat_\theta(z_i)$ is continuously differentiable. The bound on $\nabla P$ additionally assumes $\norm{D_i(\theta')}\le G$ along the segment from $\theta_{\mathrm{old}}$ to $\theta$. Remark~\ref{rem:draft} assumes an $L_R$-Lipschitz reward gradient along the segment from $\xhat_i^{\mathrm{old}}$ to $x_i$.
\item \textnormal{Transfer model} (Proposition~\ref{prop:transfer} only). The step starts at $\theta_{\mathrm{old}}$ and uses a symmetric positive semidefinite preconditioner $M$, fixed conditional on $\mathcal A$ and the selected lengths. Gradients satisfy the shared-mean and conditional-independence assumptions stated below. These assumptions are not established for the implemented optimizer; AdamW and gradient clipping are not covered.
\end{enumerate}

\subsection{Verified target selection}\label{app:prox}
\newcommand{\mendStateTarget}{%
\begin{enumerate}[label=(\roman*), leftmargin=1.8em, itemsep=1pt, topsep=1pt]
\item Assume (A1) and (A2), and fix a seed with cap $\kappa$.
\item Its capped reward gain bounds its quadratic displacement cost:
\[
\Rk(\ystar)-\Rk(x)\ge\frac{\norm{\ystar-x}^2}{2\tau}\ge0.
\]
The first inequality is strict whenever $\ystar\ne x$.
\item The displacement is bounded by both the longest proposal and the remaining reward below the cap:
\[
\norm{\ystar-x}\le\min\big\{\eta_K,\sqrt{2\tau(\kappa-\Rk(x))}\big\}.
\]
\item The raw reward satisfies the same lower bound:
\[
R(\ystar)-R(x)\ge\frac{\norm{\ystar-x}^2}{2\tau}.
\]
\end{enumerate}}
\ifdefined\mendappxstandalone
\begin{proposition}[Verified target selection]\label{prop:target}\label{prop:target-app}
\mendStateTarget
\end{proposition}
\else
\renewcommand{\mendrestatename}{Proposition~\ref{prop:target}, full statement}
\begin{mendrestate}[Verified target selection]
\mendStateTarget
\end{mendrestate}
\fi

Write $r(x)=\sqrt{2\tau(\kappa-\Rk(x))}$, suppressing its dependence on the seed's cap.

\begin{corollary}[Averaged form]\label{cor:w2}
\begin{enumerate}[label=(\roman*), leftmargin=1.8em, itemsep=1pt, topsep=1pt]
\item Assume (A1) to (A3), with $\pi$ and $\pi'$ the laws of $x$ and $\ystar$.
\item The mean capped gain bounds the mean squared displacement and the quadratic transport cost:
\[
\E[\Rk(\ystar)-\Rk(x)]
\ge\frac{1}{2\tau}\E\norm{\ystar-x}^2
\ge\frac{1}{2\tau}\Wtwo^2(\pi,\pi').
\]
\end{enumerate}
\end{corollary}

\begin{proof}[Proof of Proposition~\ref{prop:target}]
Since $x$ is a candidate, $J(\ystar)\ge J(x)=\Rk(x)$, strictly for a move. Rearranging gives
\[
\frac{\norm{\ystar-x}^2}{2\tau}
\le\Rk(\ystar)-\Rk(x)
\le\kappa-\Rk(x).
\]
Thus $\norm{\ystar-x}\le r(x)$. Every proposal has length $\eta_j\le\eta_K$, giving the other bound. For raw reward, samples at or above the cap are kept and both sides vanish. Otherwise $\Rk(x)=R(x)$ and $R(\ystar)\ge\Rk(\ystar)$, which gives (iv).
\end{proof}

\begin{proof}[Proof of Corollary~\ref{cor:w2}]
The capped gain is nonnegative, and $\norm{\ystar-x}^2\le\eta_K^2$. Taking expectations in Proposition~\ref{prop:target} gives the first inequality, allowing an infinite expected gain. The joint law of $(x,\ystar)$ couples $\pi$ and $\pi'$, so its cost bounds the infimum over all couplings. For a finite round, this coupling is $n^{-1}\sum_i\delta_{(x_i,\ystar_i)}$.
\end{proof}

\begin{remark}[The update is not proximal]\label{rem:notprox}
Proposition~\ref{prop:target} concerns targets, not a proximal parameter update. An AdamW step need not realize their displacements or respect their bounds, and shared parameters can change kept samples as well as moved ones (Appendix~\ref{app:choices}).
\end{remark}

\paragraph{Scope.} The guarantees apply to selected targets under the training reward, not to held-out evaluators or the trained model. For a fixed prompt and cap, allowing every latent as a candidate gives the proximal problem $\arg\max_y\{\Rk(y)-\norm{y-x}^2/(2\tau)\}$, the pointwise problem associated with a JKO step for the potential energy $-\E\Rk$ \citep{jko1998}. The finite candidate rule never does worse than staying put; no accuracy guarantee relative to the unrestricted optimum is claimed.

\subsection{First-order form of the update}\label{app:firstorder}
\newcommand{\mendStateFirstorder}{%
\begin{enumerate}[label=(\roman*), leftmargin=1.8em, itemsep=2pt, topsep=1pt]
\item Assume (A1), (A2) and (A4). Define $\ell_i(\theta)=\ip{\hat h_i}{\xhat_\theta(z_i)}$, $e_i(\theta)=\xhat_\theta(z_i)-\xhat_i^{\mathrm{old}}$ and $P(\theta)=\sum_i w_i\norm{e_i(\theta)}^2$.
\item For every $\theta$, the loss separates into a proximity term and the accepted seeds' hint projections:
\[
\mathcal L(\theta)=P(\theta)-\frac{2}{|\mathcal A|}\sum_{i\in\mathcal A}\eta_i\ell_i(\theta)+C,
\qquad
C=\sum_i w_i\big(2\ip{\xhat_i^{\mathrm{old}}}{d_i}+\norm{d_i}^2\big).
\]
Its negative gradient is
\[
\begin{aligned}
-\nabla\mathcal L(\theta)
&=\frac{2}{|\mathcal A|}\sum_{i\in\mathcal A}\frac{\eta_i}{\norm{g_i}}
\nabla_\theta\ip{g_i}{\xhat_\theta(z_i)}-\nabla P(\theta),\\
\nabla P(\theta)&=2\sum_i w_i D_i(\theta)^*e_i(\theta).
\end{aligned}
\]
\item The proximity gradient vanishes when all $e_i(\theta)=0$, in particular at $\theta_{\mathrm{old}}$. Under the Jacobian bound in (A4),
\[
\norm{\nabla P(\theta)}_\Theta
\le2(1+\lambda_{\mathrm{keep}})G^2\norm{\theta-\theta_{\mathrm{old}}}_\Theta.
\]
\end{enumerate}}
\newcommand{\mendStateTransfer}{%
\begin{enumerate}[label=(\roman*), leftmargin=1.8em, itemsep=1pt, topsep=1pt]
\item Assume (A1), (A2), (A4) and (A5), with $\Delta\theta=-\alpha M\nabla\mathcal L(\theta_{\mathrm{old}})$ and $\alpha>0$. Conditional on $\mathcal A$ and the selected lengths, suppose the gradients $q_s=\nabla\ell_s(\theta_{\mathrm{old}})$ of accepted seeds and a held-out seed $o\notin\mathcal A$ satisfy
\[
q_s=m+\xi_s,\qquad \E\xi_s=0,\qquad \E\norm{\xi_s}_\Theta^2\le\sigma^2.
\]
Here $m$ and $M$ are fixed, the residuals are independent, and accepted and held-out seeds share the same conditional mean $m$. The held-out seed is also rolled out by $\theta_{\mathrm{old}}$. Write $\bar\eta=|\mathcal A|^{-1}\sum_{i\in\mathcal A}\eta_i$; all expectations below use this conditioning.
\item The expected first-order change in the held-out hint projection depends only on the shared component:
\[
\E\ip{q_o}{\Delta\theta}_\Theta=2\alpha\bar\eta\,m^\top Mm\ge0.
\]
\item The step consists of a shared component and a zero-mean residual:
\[
\begin{gathered}
\Delta\theta=2\alpha\bar\eta Mm+s,
\qquad s=\frac{2\alpha}{|\mathcal A|}M\sum_{i\in\mathcal A}\eta_i\xi_i,\\
\E\norm{s}_\Theta^2\le\frac{4\alpha^2\norm{M}^2\eta_K^2\sigma^2}{|\mathcal A|}.
\end{gathered}
\]
\item For each accepted seed $k\in\mathcal A$, its expected first-order change exceeds the held-out value by at most
\[
0\le\E\ip{q_k}{\Delta\theta}_\Theta-\E\ip{q_o}{\Delta\theta}_\Theta
\le\frac{2\alpha\eta_K\norm{M}\sigma^2}{|\mathcal A|}.
\]
\end{enumerate}}
\ifdefined\mendappxstandalone
\begin{theorem}[First-order realization]\label{thm:firstorder}\label{prop:firstorder}
\mendStateFirstorder
\end{theorem}
\else
\renewcommand{\mendrestatename}{Proposition~\ref{prop:firstorder}, full statement}
\begin{mendrestate}[First-order realization]
\mendStateFirstorder
\end{mendrestate}
\fi
\begin{proposition}[Transfer of the step to held-out seeds]\label{prop:transfer}
\mendStateTransfer
\end{proposition}
Since $\ip{q_s}{\Delta\theta}_\Theta=\ip{\hat h_s}{D_s(\theta_{\mathrm{old}})\Delta\theta}$, Proposition~\ref{prop:transfer} concerns the linearized projection of a clean prediction onto its endpoint hint, not the change in endpoint reward or a held-out evaluator.

\begin{proof}[Proof of the first-order realization result]
By (A1), $\xhat_i^{\mathrm{old}}$ and $d_i$ are constant with respect to $\theta$. Expanding each squared error gives
\[
\norm{e_i(\theta)-d_i}^2
=\norm{e_i(\theta)}^2-2\ip{\xhat_\theta(z_i)}{d_i}
+2\ip{\xhat_i^{\mathrm{old}}}{d_i}+\norm{d_i}^2.
\]
Sum with weights $w_i$ and substitute $d_i=\eta_i\hat h_i$ on $\mathcal A$ and $d_i=0$ elsewhere to obtain the loss identity. Differentiating gives (ii), since $\hat h_i=g_i/\norm{g_i}$ on $\mathcal A$ and the derivative of $\norm{e_i(\theta)}^2$ is $2D_i(\theta)^*e_i(\theta)$. This derivative vanishes at $\theta_{\mathrm{old}}$.

For (iii), the mean value inequality gives $\norm{e_i(\theta)}\le G\norm{\theta-\theta_{\mathrm{old}}}_\Theta$. Since $\norm{D_i(\theta)^*}\le G$,
\[
\norm{\nabla P(\theta)}_\Theta
\le2G^2\norm{\theta-\theta_{\mathrm{old}}}_\Theta\sum_i w_i
\le2(1+\lambda_{\mathrm{keep}})G^2\norm{\theta-\theta_{\mathrm{old}}}_\Theta.
\]
The weight sum is $1+\lambda_{\mathrm{keep}}$ when both subsets are nonempty, $1$ when all seeds move, and $\lambda_{\mathrm{keep}}$ when none move.
\end{proof}

\begin{proof}[Proof of Proposition~\ref{prop:transfer}]
At $\theta_{\mathrm{old}}$, the proximity gradient vanishes, giving
\[
\Delta\theta=\frac{2\alpha}{|\mathcal A|}\sum_{i\in\mathcal A}\eta_i Mq_i.
\]
All quantities below are conditional on $\mathcal A$ and the selected lengths. Finite second moments make the products integrable. Independence and zero means give
\[
\E\ip{m}{M\xi_s}_\Theta=0,
\qquad
\E\ip{\xi_s}{M\xi_{s'}}_\Theta=0\quad(s\ne s'),
\]
while positive semidefiniteness gives $0\le\xi_s^\top M\xi_s\le\norm{M}\norm{\xi_s}_\Theta^2$.

For (ii), the held-out residual is independent of every accepted residual, so $\E\ip{q_o}{Mq_i}_\Theta=m^\top Mm$. Summing yields $\E\ip{q_o}{\Delta\theta}_\Theta=2\alpha\bar\eta\,m^\top Mm\ge0$.

For (iii), substitute $q_i=m+\xi_i$ into the step. The residual $s$ has zero mean, and its cross terms vanish, giving
\[
\E\norm{s}_\Theta^2
\le\frac{4\alpha^2\norm{M}^2}{|\mathcal A|^2}
\sum_{i\in\mathcal A}\eta_i^2\E\norm{\xi_i}_\Theta^2
\le\frac{4\alpha^2\norm{M}^2\eta_K^2\sigma^2}{|\mathcal A|}.
\]
For (iv), only the self-term $i=k$ differs from the held-out calculation:
\[
\E\ip{q_k}{\Delta\theta}_\Theta
=2\alpha\bar\eta\,m^\top Mm
+\frac{2\alpha\eta_k}{|\mathcal A|}\E[\xi_k^\top M\xi_k].
\]
The final term lies between $0$ and $2\alpha\eta_K\norm{M}\sigma^2/|\mathcal A|$.
\end{proof}

\begin{remark}[Relation to one-step reward backpropagation]\label{rem:draft}
Let $D_i=D_i(\theta_{\mathrm{old}})$. The accepted-seed term uses $D_i^*\nabla R(x_i)$, whereas one-step reward backpropagation \citep{xu2023imagereward,clark2024draft} uses $D_i^*\nabla R(\xhat_i^{\mathrm{old}})$. Under the Lipschitz condition in (A4),
\[
\norm{D_i^*\big(\nabla R(x_i)-\nabla R(\xhat_i^{\mathrm{old}})\big)}_\Theta
\le\norm{D_i}L_R\norm{x_i-\xhat_i^{\mathrm{old}}}.
\]
Multiplying by $2\eta_i/(|\mathcal A|\norm{g_i})$ gives the discrepancy between the corresponding weighted gradient terms. The bound is qualitative: the endpoint-to-prediction gap is not assumed small.
\end{remark}

\paragraph{The EMA lag.} The implemented step starts at $\theta$, not $\theta_{\mathrm{old}}$, so its loss gradient includes the proximity term. Let $\Gamma_u=\theta-\theta_{\mathrm{old}}$ after update $u$ and the behavior EMA, and let $\Delta\theta_u$ be that update. The recursion $\Gamma_u=\mu_u(\Gamma_{u-1}+\Delta\theta_u)$ gives
\[
\norm{\Gamma_u}_\Theta
\le\Big(\prod_{v=1}^u\mu_v\Big)\norm{\Gamma_0}_\Theta
+\frac{\bar\mu}{1-\bar\mu}\max_{1\le v\le u}\norm{\Delta\theta_v}_\Theta
\]
whenever $0\le\mu_v\le\bar\mu<1$. With zero initial lag and $\bar\mu=0.1$, the lag is at most one ninth of the largest step over the updates considered. Proposition~\ref{prop:firstorder}(iii) bounds the proximity gradient by $2(1+\lambda_{\mathrm{keep}})G^2\norm{\Gamma_u}_\Theta$. This term anchors predictions to the behavior adapter, not the base model.

\paragraph{Interpreting the update.} At $\theta_{\mathrm{old}}$, the descent direction uses reward gradients evaluated at rollout endpoints, normalized in latent space, and filtered and scaled by the verdict. For the idealized step of Proposition~\ref{prop:transfer}, writing $D_s=D_s(\theta_{\mathrm{old}})$ gives
\[
D_s\Delta\theta=\frac{2\alpha}{|\mathcal A|}\sum_{i\in\mathcal A}D_sMD_i^*d_i.
\]
Thus the linearized prediction change is a kernel-weighted combination of accepted displacements. Proposition~\ref{prop:transfer} describes its expected transfer under (A5).

\subsection{Target mass across region boundaries}\label{app:modes}
\begin{corollary}[Mode mass of the targets]\label{thm:modes}
\begin{enumerate}[label=(\roman*), leftmargin=1.8em, itemsep=1pt, topsep=1pt]
\item Assume (A1) to (A3). Let $\rho(x)=\min\{\eta_K,r(x)\}$ and fix a Borel set $A\subseteq\R^D$.
\item The change in probability assigned to $A$ satisfies
\[
|\pi'(A)-\pi(A)|
\le\Pr\big[\mathrm{dist}(x,\partial A)\le\norm{\ystar-x}\big]
\le\Pr\big[\mathrm{dist}(x,\partial A)\le\rho(x)\big].
\]
\item A region can receive targets only from samples within their displacement bound of it:
\[
\pi'(A)\le\Pr\big[\mathrm{dist}(x,A)\le\rho(x)\big].
\]
\end{enumerate}
\end{corollary}

\begin{proof}
The distance functions are 1-Lipschitz for nonempty sets and identically $+\infty$ otherwise, so the events are measurable by (A3). Under the seed coupling,
\[
\pi'(A)-\pi(A)
=\Pr[\ystar\in A,x\notin A]-\Pr[x\in A,\ystar\notin A].
\]
Its absolute value is at most the probability that exactly one endpoint belongs to $A$. In that event, the segment from $x$ to $\ystar$ meets $\partial A$: otherwise the disjoint open sets $\mathrm{int}\,A$ and $\mathrm{int}(A^c)$ would disconnect the segment. Hence $\mathrm{dist}(x,\partial A)\le\norm{\ystar-x}\le\rho(x)$, proving (ii). Finally, $\ystar\in A$ implies $\mathrm{dist}(x,A)\le\norm{\ystar-x}\le\rho(x)$, proving (iii).
\end{proof}

Samples at the cap have $\rho(x)=0$, and regions outside every sample's displacement bound receive no target mass. In contrast, consider the KL tilt $\pi_\beta(dx)\propto e^{R(x)/\beta}\pi(dx)$, with $\beta>0$ and finite normalizer. For $\pi(A)>0$,
\[
\frac{\pi_\beta(A)}{\pi(A)}
=\frac{\E_\pi[e^{R/\beta}\mid A]}{\E_\pi[e^{R/\beta}]}.
\]
If $R\le r_A$ on $A$ and $R\ge r_A+\Delta$ off $A$, then
\[
\frac{\pi_\beta(A)}{\pi(A)}
\le\frac{1}{\pi(A)+(1-\pi(A))e^{\Delta/\beta}},
\]
regardless of the distance between $A$ and the remaining support. These are target-level statements; diversity after training is evaluated empirically.
