# Supplementary material for: MEND: RL For Flow Models via Proximal Velocity Matching
Source: arXiv:2610.05954 source file (2026-10-05)
Supplement: Supplementary file 4 [file v2_D_results.tex]

\section{Full result tables}\label{app:results}\label{app:exp}
Table~\ref{tab:main-full} extends Table~\ref{tab:main} with every evaluator, diversity, distance to the base and 95\% intervals.
\input{appendix/v2_ci_macros}
\newcommand{\ciCell}[2]{{\scriptsize\textcolor{gray}{[\res{appxci.#1.#2.lo}, \res{appxci.#1.#2.hi}]}}}
\newcommand{\ciRow}[1]{\multicolumn{4}{@{}r}{\scriptsize\textcolor{gray}{95\% interval}} & \ciCell{#1}{pick} & \ciCell{#1}{hps2} & \ciCell{#1}{hps3} & \ciCell{#1}{ir} & \ciCell{#1}{clip} & \ciCell{#1}{aes} & \ciCell{#1}{div} & \ciCell{#1}{dist} \\}
\newcommand{\ciRowBase}[1]{\multicolumn{4}{@{}r}{\scriptsize\textcolor{gray}{95\% interval}} & \ciCell{#1}{pick} & \ciCell{#1}{hps2} & \ciCell{#1}{hps3} & \ciCell{#1}{ir} & \ciCell{#1}{clip} & \ciCell{#1}{aes} & \ciCell{#1}{div} & {\scriptsize\textcolor{gray}{n/a}} \\}
\begin{table}[!h]
\centering
\caption{\textbf{Full SD3.5-M results.} DrawBench $200\times5$; setting is training/evaluation guidance, $^\dagger$ marks rows from \citet{zhou2026opsd} (n/r: not reported) and $^\ast$ the default Adam $\epsilon$. Grey sub-rows give 95\% prompt-bootstrap intervals; \best{bold} and \second{underline} mark the best and second best trained headline rows.}
\label{tab:main-full}
\footnotesize
\setlength{\tabcolsep}{2pt}
\resizebox{\linewidth}{!}{%
\begin{tabular}{lccccccccccc}
\toprule
\headrow Method & Upd. & Setting & Reg. & PickScore & HPSv2.1 & HPSv3 & ImageReward & CLIPScore & Aesthetic & Div.\,$\uparrow$ & Dist.\,$\downarrow$ \\
\midrule
\rowcolor{tabgroup}[0pt][0pt] \multicolumn{12}{@{}l}{\textnormal{Headline settings (Appendix~\ref{app:settings})}} \\
SD3.5-M & 0 & --/4.5 & & 22.35 & 0.280 & 2.72 & 0.83 & 0.283 & 5.39 & 0.325 & 0 \\
\ciRowBase{base45}
\begin{tabular}[c]{@{}l@{}}Flow-GRPO,\\PickScore adapter\end{tabular} & ${\sim}$4k & 4.5/4.5 & KL & 23.52 & 0.316 & 7.04 & 1.27 & 0.280 & \second{5.90} & \best{0.202} & \best{0.313} \\
\ciRow{fg}
\begin{tabular}[c]{@{}l@{}}DiffusionNFT,\\multi-reward\end{tabular} & 1.7k & 1/1 & MSE & \best{23.82} & \best{0.331} & \best{7.50} & \best{1.49} & \best{0.292} & \best{6.02} & 0.130 & 0.538 \\
\ciRow{nft}
\oursrow \textbf{\mend{} (ours)} & 100 & 1/4.5 & none & \second{\res{cfg45.pick}} & \second{\res{cfg45.hps2}} & \second{\res{cfg45.hps3}} & \second{\res{cfg45.ir}} & \second{\res{cfg45.clip}} & \res{cfg45.aes} & \second{\res{cfg45.div}} & \best{\res{cfg45.dist}} \\
\ciRow{cfg45}
\midrule
\rowcolor{tabgroup}[0pt][0pt] \multicolumn{12}{@{}l}{\textnormal{Matched 100-update comparison (Protocol~O)}} \\
SD3.5-M & 0 & --/1 & & 20.58 & 0.207 & $-6.44$ & $-0.52$ & 0.239 & 5.14 & 0.578 & 0 \\
\ciRowBase{base1}
\oursrow \mend{} & 100 & 1/1 & none & \resrow{fin} \\
\ciRow{fin}
\oursrow \mend{}, default Adam $\epsilon^\ast$ & 100 & 1/1 & none & \iPick & \iHPSt & \iHPSthree & \iIR & \iClip & \iAes & \iDiv & \iDist \\
ReFL$^\dagger$ & 100 & 1/1 & none & 23.92 & n/r & n/r & n/r & n/r & n/r & n/r & n/r \\
DiffusionNFT$^\dagger$ & 100 & 1/1 & MSE & 23.43 & n/r & n/r & n/r & n/r & n/r & n/r & n/r \\
\bottomrule
\end{tabular}}
\end{table}
\subsection{Validation split}\label{app:setup}
Every design decision was made at the development budget on DrawBench prompts 1 to 64. Table~\ref{tab:clean} repeats Table~\ref{tab:main} on DrawBench prompts 65 to 200, which no decision has seen.

\begin{table}[!htbp]
\centering
\caption{\textbf{Held-out DrawBench prompts 65 to 200.} Rows at guidance 4.5 reuse the $136\times5$ images of Table~\ref{tab:main}; other rows use $136\times2$ images. HF is a ratio to SD3.5-M at guidance 4.5 and is not ranked.}
\label{tab:clean}
\small
\setlength{\tabcolsep}{3pt}
\resizebox{\linewidth}{!}{%
\begin{tabular}{lccccccccc}
\toprule
\headrow Method & Setting & PickScore & HPSv2.1 & HPSv3 & ImageReward & CLIPScore & Aesthetic & Div. & HF \\
\midrule
SD3.5-M & 1 & 20.62 & 0.209 & $-6.58$ & $-0.49$ & 0.239 & 5.16 & \best{0.568} & 0.40 \\
SD3.5-M & 4.5 & 22.39 & 0.283 & 2.85 & 0.87 & 0.284 & 5.43 & 0.321 & 1.00 \\
Flow-GRPO, PickScore adapter & 4.5 & 23.52 & 0.317 & 7.03 & 1.31 & 0.281 & 5.95 & 0.201 & 0.96 \\
DiffusionNFT, multi-reward & 1 & 23.81 & \best{0.332} & \best{7.37} & \best{1.53} & \best{0.293} & 6.04 & 0.128 & 0.56 \\
\oursrow \mend{} & 4.5 & \resrowhf{ccfg45} \\
\oursrow \mend{} & 1 & \best{\res{cfin.pick}} & \res{cfin.hps2} & \res{cfin.hps3} & \res{cfin.ir} & \res{cfin.clip} & \best{\res{cfin.aes}} & \res{cfin.div} & \res{cfin.hf} \\
\oursrow \mend{}, default Adam $\epsilon$ & 1 & 23.98 & 0.301 & 3.90 & 1.14 & 0.274 & 6.22 & 0.195 & 0.48 \\
\bottomrule
\end{tabular}}
\end{table}
