# Supplementary material for: MEND: RL For Flow Models via Proximal Velocity Matching
Source: arXiv:2610.05954 source file (2026-10-05)
Supplement: Supplementary file 5 [file v2_E_dynamics.tex]

\section{Training dynamics and other backbones}\label{app:dynamics}\label{app:campaign}\label{app:curves}
\begin{figure}[!htbp]
\centering
\includegraphics[width=\linewidth]{figures/v2_appx/fig_perreward.pdf}
\caption{\textbf{Held-out reward and diversity for each training reward.} Single-seed \mend{} runs on DrawBench $200\times5$; ReFL and DiffusionNFT curves follow \citet[Figure~8]{zhou2026opsd}, and open triangles mark DiffusionNFT under Protocol~O in our pipeline.}
\label{fig:perreward}\label{fig:campaign-perreward}
\end{figure}
Figure~\ref{fig:perreward} follows the per-reward runs of Section~\ref{sec:rewards} through training.
\label{app:campaign-curves}
\subsection{Other rewards and SD3-M}\label{app:rewards}
Table~\ref{tab:rewards} holds one run per training reward and Table~\ref{tab:sd3m} the run on SD3-M. The $^\ddagger$ row gives, for each run, the last update before a held-out evaluator on val64 falls below its best earlier value by more than its 95\% paired bootstrap half-width, a rule fixed before the numbers were read.

\begin{table}[!htbp]
\centering

\centering
\caption{\textbf{One run per training reward.} SD3.5-M, Protocol~O, update 100, DrawBench $200\times5$; $^\dagger$: from \citet{zhou2026opsd}, $^\ast$: default Adam $\epsilon$, $^\ddagger$: last update before held-out decline. The HPSv3 run is in Table~\ref{tab:rewards-full}.}
\label{tab:rewards}
\small
\setlength{\tabcolsep}{2.5pt}
\begin{tabular}{@{}lccccc@{}}
\toprule
\headrow Method & PickScore & CLIPScore & HPSv2.1 & HPSv3 & ImageReward \\
\midrule
SD3.5-M$^\dagger$ & 20.51 & 0.237 & 0.204 & $-6.47$ & $-0.58$ \\
SD3.5-M, measured by us & 20.58 & 0.239 & 0.207 & $-6.44$ & $-0.52$ \\
ReFL$^\dagger$ & 23.92 & 0.308 & 0.358 & 9.33 & 1.28 \\
DiffusionNFT$^\dagger$ & 23.43 & 0.298 & 0.336 & 9.14 & 1.46 \\
\oursrow \mend{} & \mPick & \res{rwclipscore.clip} & \res{rwhpsv2.hps2} & -- & \res{rwimagereward.ir} \\
\oursrow \mend{}, default $\epsilon^\ast$ & \iPick & \res{rwdefclipscore.clip} & \res{rwdefhpsv2.hps2} & -- & \res{rwdefimagereward.ir} \\
\oursrow \mend{}, before decline$^\ddagger$ & -- & \res{rwclippre.clip} & \res{rwhpsv2pre.hps2} & -- & \res{rwirpre.ir} \\
\bottomrule
\end{tabular}
\end{table}
\begin{table}[!htbp]
\centering

\centering
\caption{\textbf{\mend{} on SD3-M.} DrawBench $200\times5$, Protocol~O, update 100; Linear-DPO is the checkpoint of \citet{li2026lineardpo}.}
\label{tab:sd3m}
\small
\setlength{\tabcolsep}{2.5pt}
\begin{tabular}{@{}lccccc@{}}
\toprule
\headrow Model & PickScore & HPSv2.1 & CLIPScore & Div.\,$\uparrow$ & Dist.\,$\downarrow$ \\
\midrule
SD3-M & 20.36 & 0.215 & 0.234 & 0.552 & 0 \\
Linear-DPO & 20.96 & 0.256 & 0.241 & 0.464 & 0.341 \\
\oursrow \mend{}, PickScore & \res{sd3mend.pick} & \res{sd3mend.hps2} & 0.263 & 0.239 & 0.500 \\
\bottomrule
\end{tabular}

\end{table}
\subsection{Every evaluator per run}\label{app:campaign-rewards}
Table~\ref{tab:rewards-full} scores each single-reward run with every evaluator, including a fifth run on HPSv3 whose last full evaluation is update 90.

\begin{table}[!htbp]
\centering
\caption{\textbf{Every evaluator for each single-reward run.} DrawBench $200\times5$; the training reward of each row is its diagonal entry. Top block at guidance 1, bottom block at guidance 4.5.}
\label{tab:rewards-full}
\small
\setlength{\tabcolsep}{3pt}
\resizebox{\linewidth}{!}{%
\begin{tabular}{lcccccccc}
\toprule
\headrow Training reward & PickScore & HPSv2.1 & HPSv3 & ImageReward & CLIPScore & Aesthetic & Div.\,$\uparrow$ & Dist.\,$\downarrow$ \\
\midrule
none (SD3.5-M) & 20.58 & 0.207 & $-6.44$ & $-0.52$ & 0.239 & 5.14 & 0.578 & 0 \\
PickScore (seed 1) & \resrow{fin} \\
CLIPScore & \resrow{rwclipscore} \\
HPSv2.1 & \resrow{rwhpsv2} \\
ImageReward & \resrow{rwimagereward} \\
HPSv3 (update 90) & \resrow{rwhpsv3} \\
\midrule
\grouprow \multicolumn{9}{l}{Headline evaluation settings (Appendix~\ref{app:settings})} \\
PickScore (seed 1) & \resrow{cfg45} \\
CLIPScore & \resrow{rwclipscore45} \\
HPSv2.1 & \resrow{rwhpsv245} \\
ImageReward & \resrow{rwimagereward45} \\
\bottomrule
\end{tabular}}
\end{table}

\subsection{Training past the budget and over-optimization}\label{app:overopt}
Trained on PickScore for 200 updates (Table~\ref{tab:overopt}, top; Figure~\ref{fig:campaign-overopt}), \mend{} keeps raising the trained reward while held-out gains flatten and diversity declines slowly. Trained on the LAION aesthetic predictor, a reward known to be over-optimized \citep{black2023ddpo,clark2024draft}, it raises the aesthetic score from 5.2 to 9.7 while every other evaluator collapses (Table~\ref{tab:overopt}, bottom).

The verdict certifies against the training reward only, so it cannot prevent this. Continuing the HPSv2.1 run from update 100 to 200 likewise raises HPSv2.1 while held-out HPSv3 falls, consistent with the $^\ddagger$ row of Table~\ref{tab:rewards}.

\begin{table}[!htbp]
\centering
\caption{\textbf{200 updates at the development budget.} DrawBench prompts 65 to 200 $\times$ 2 seeds. Top: PickScore training; bottom: LAION aesthetic training.}
\label{tab:overopt}
\small
\setlength{\tabcolsep}{4pt}
\begin{tabular}{llccccccc}
\toprule
\headrow Training reward & Updates & PickScore & HPSv3 & ImageReward & CLIPScore & Aesthetic & Div. & Dist. \\
\midrule
none (SD3.5-M) & 0 & 20.62 & $-6.58$ & $-0.49$ & 0.239 & 5.16 & 0.568 & 0 \\
\midrule
\oursrow PickScore & 50 & 23.15 & 2.93 & 0.81 & 0.262 & 6.15 & 0.271 & 0.457 \\
\oursrow & 100 & 23.47 & 3.02 & 0.95 & 0.265 & 6.21 & 0.252 & 0.469 \\
\oursrow & 150 & 23.65 & 3.31 & 0.99 & 0.266 & 6.28 & 0.240 & 0.476 \\
\oursrow & 200 & 23.78 & 3.34 & 1.04 & 0.270 & 6.22 & 0.238 & 0.474 \\
\midrule
Aesthetic & 50 & 19.90 & $-5.90$ & $-0.84$ & 0.155 & 8.84 & 0.200 & 0.634 \\
 & 100 & 18.91 & $-6.28$ & $-1.27$ & 0.123 & 9.35 & 0.198 & 0.677 \\
 & 150 & 18.58 & $-6.76$ & $-1.48$ & 0.107 & 9.53 & 0.185 & 0.695 \\
 & 200 & 18.43 & $-6.71$ & $-1.56$ & 0.099 & 9.66 & 0.192 & 0.703 \\
\bottomrule
\end{tabular}
\end{table}

\input{figures/snippets/v2_fig_overopt}

\subsection{Z-Image-Turbo}\label{app:campaign-zimage}
Z-Image-Turbo \citep{cai2025zimage} is a distilled model sampled in 9 steps at 1024 pixels; we follow \citet[Appendix~C.1]{zhou2026opsd} with 1024-pixel rollouts and $48\times12$ images per update. Both runs improve every held-out evaluator except CLIPScore (Table~\ref{tab:zimage-full}).

\begin{table}[!htbp]
\centering
\caption{\textbf{Z-Image-Turbo, every evaluator.} DrawBench $200\times5$, 1024 pixels, 9 steps.}
\label{tab:zimage-full}\label{tab:zimage}
\small
\setlength{\tabcolsep}{3pt}
\resizebox{\linewidth}{!}{%
\begin{tabular}{lcccccccc}
\toprule
\headrow Model & PickScore & HPSv2.1 & HPSv3 & ImageReward & CLIPScore & Aesthetic & Div.\,$\uparrow$ & Dist.\,$\downarrow$ \\
\midrule
Z-Image-Turbo & \resrow{zbase} \\
\oursrow \mend{}, trained on PickScore & \resrow{zpick} \\
\oursrow \mend{}, trained on HPSv2.1 & \resrow{zhps} \\
\bottomrule
\end{tabular}}
\end{table}
