# Supplementary material for: MEND: RL For Flow Models via Proximal Velocity Matching
Source: arXiv:2610.05954 source file (2026-10-05)
Supplement: Supplementary file 6 [file v2_F_ablations.tex]

\section{Ablations and controls}\label{app:ablations}
Table~\ref{tab:abl-more} varies one part of \mend{} at a time at the development budget; ``fixed length'' rescales every trained move to RMS 0.1, and ``self-normalized loss'' divides each seed's error by the squared length of its move. A looser cap, a price band with more acceptances and a higher learning rate all trade diversity for reward.

\begin{table}[!htbp]
\centering
\caption{\textbf{Development budget ablations.} SD3.5-M, $16\times8$ images per update, 50 updates, one training seed per arm; last two columns on DrawBench $200\times5$ where measured. Moved: mean share of seeds receiving a move target.}
\label{tab:abl-more}\label{tab:ablation}
\small
\setlength{\tabcolsep}{3pt}
\resizebox{\linewidth}{!}{%
\begin{tabular}{llccccccc}
\toprule
\headrow & & & \multicolumn{4}{c}{DrawBench 1 to 64 $\times$ 2 (development)} & \multicolumn{2}{c}{DrawBench $200 \times 5$} \\
\cmidrule(lr){4-7}\cmidrule(lr){8-9}
\headrow & Arm & Moved & PickScore & HPSv3 & ImageReward & Div. & PickScore & Div. \\
\midrule
& SD3.5-M, no update & n/a & 20.52 & $-6.77$ & $-0.58$ & 0.589 & \res{abbase.pick} & \res{abbase.div} \\
\oursrow & \mend{} (explicit candidates; verdict, price, cap; single state; certified move) & 0.34 & 22.99 & 3.03 & 0.66 & 0.318 & \res{abref.pick} & \res{abref.div} \\
\oursrow & \mend{}, $\epsilon = 10^{-12}$ & 0.34 & 23.10 & 3.12 & 0.76 & 0.292 & -- & -- \\
\midrule
\multirow{5}{*}{\rotatebox{90}{\footnotesize candidates}} & One candidate ($K = 1$, $\eta = 0.1$) & 0.37 & 23.03 & 3.33 & 0.71 & 0.302 & \res{abkone.pick} & \res{abkone.div} \\
& Two states in $[0.2, 0.6]$, $\eta \in \{0.05, 0.1, 0.2\}$ & 0.37 & 22.88 & 3.16 & 0.68 & 0.335 & -- & -- \\
& Anchored restart proposals from $t = 0.86$ & 0.41 & 22.79 & 2.48 & 0.67 & 0.316 & -- & -- \\
& Two gradient steps per proposal & 0.36 & 22.98 & 2.01 & 0.65 & 0.292 & -- & -- \\
& Reward gradient clipped to unit norm & 0.35 & 23.18 & 3.17 & 0.73 & 0.293 & -- & -- \\
\midrule
\multirow{7}{*}{\rotatebox{90}{\footnotesize verdict, cap}} & No price ($\tau = \infty$): best capped reward wins & 0.78 & 23.05 & 2.96 & 0.67 & 0.310 & \res{abnoprice.pick} & \res{abnoprice.div} \\
& No cap ($\kappa = \infty$), verdict on & 0.45 & 23.17 & 3.24 & 0.74 & 0.304 & \res{abnocap.pick} & \res{abnocap.div} \\
& Price band $[0.6, 0.8]$ & 0.54 & 23.09 & 3.32 & 0.72 & 0.297 & -- & -- \\
& Cap quantile $q = 0.9$ & 0.42 & 23.03 & 3.48 & 0.72 & 0.300 & -- & -- \\
& No per-seed verdict: every seed below the cap takes $\eta = 0.2$ & 0.81 & 23.35 & 3.60 & 0.81 & 0.264 & \res{abnvtwo.pick} & \res{abnvtwo.div} \\
& No per-seed verdict: every seed below the cap takes $\eta = 0.1$ & 0.81 & 23.00 & 2.92 & 0.66 & 0.316 & \res{abnvone.pick} & \res{abnvone.div} \\
& Endpoint check only: one $\eta = 0.2$ candidate kept iff $R(y) > R(x)$; no price, no cap & 0.83 & 23.22 & 3.52 & 0.76 & 0.299 & \res{abendpoint.pick} & \res{abendpoint.div} \\
\midrule
\multirow{5}{*}{\rotatebox{90}{\footnotesize target}} & No verdict, no cap, fixed length 0.1 on every seed, self-normalized loss & 1.00 & 23.59 & 3.51 & 0.95 & 0.216 & -- & -- \\
& \quad same, two states, squared loss & 1.00 & 23.54 & 5.37 & 0.91 & 0.216 & -- & -- \\
& \quad + verdict and cap ($\eta \in \{0.05, 0.1, 0.2\}$) & 0.37 & 23.16 & 3.27 & 0.80 & 0.291 & -- & -- \\
& \quad\quad squared loss (fixed-length variant) & 0.37 & 23.16 & 3.52 & 0.82 & 0.299 & -- & -- \\
& Two trained states and learning rate $6 \times 10^{-4}$ (two factors change) & 0.36 & 23.12 & 3.38 & 0.76 & 0.300 & -- & -- \\
\midrule
\multirow{6}{*}{\rotatebox{90}{\footnotesize optimizer}} & Learning rate $4.5 \times 10^{-4}$ & 0.34 & 23.02 & 3.12 & 0.60 & 0.292 & -- & -- \\
& Learning rate $6 \times 10^{-4}$ & 0.34 & 23.19 & 2.81 & 0.83 & 0.277 & -- & -- \\
& \quad with cap quantile $q = 0.5$ & 0.30 & 23.10 & 2.83 & 0.72 & 0.274 & -- & -- \\
& \quad with cap quantile $q = 0.6$ & 0.31 & 23.26 & 2.83 & 0.81 & 0.280 & -- & -- \\
& \quad with cap quantile $q = 0.9$ & 0.39 & 23.31 & 3.49 & 0.83 & 0.275 & -- & -- \\
& Learning rate $10^{-3}$ & 0.34 & 23.34 & 3.49 & 0.88 & 0.269 & -- & -- \\
\bottomrule
\end{tabular}}
\end{table}

\begin{figure}[!htbp]
\centering
\includegraphics[width=\linewidth]{figures/v2_appx/fig_ablation.pdf}
\caption{\textbf{One-factor arms at the development budget.} PickScore and diversity of the arms of Table~\ref{tab:abl-more}; dotted lines mark \mend{}.}
\label{fig:abl-full}
\end{figure}
\subsection{Design choices}\label{app:choices}
Candidates are explicit moves of the endpoint, decoded and scored as they are; re-noising the endpoint and denoising again \citep{meng2022sdedit,bansal2023universal} trained less cleanly in development runs. Nearly every accepted move takes the shortest rung $\eta = \hpEtaOne$, because the longer moves lose on reward and not only on price, so the longer rungs check that the shortest move lies on the rising part of the ray.

The verdict certifies targets; the optimizer decides how far the model moves. In the two Protocol~O runs, the mean squared endpoint move of 12 held-out seeds re-rolled after each update has a median of 0.78 and 1.03 times the mean certified squared move. Seeds the verdict would keep move as much as seeds it would move, and the median projection of the move onto the certified direction is 0.001.
\subsection{Sensitivity at the full budget}\label{app:sensitivity}
Table~\ref{tab:sensitivity} varies one factor at the Protocol~O budget, stopped at update 50. A second launch of the reference differs by 0.01 PickScore, the initial price and the EMA barely matter, a 0.05 rung lowers PickScore, and adding HPSv2.1 to the reward raises HPSv2.1 and HPSv3 at no PickScore cost.

\begin{table}[!htbp]
\centering
\caption{\textbf{Sensitivity at the full budget.} Protocol~O budget, update 50, one training seed per arm, DrawBench prompts 65 to 200 $\times$ 2 seeds; last column on DrawBench $200\times5$ where measured. $\tau_{50}$: the price at update 50.}
\label{tab:sensitivity}
\small
\setlength{\tabcolsep}{3pt}
\resizebox{\linewidth}{!}{%
\begin{tabular}{lcccccccccc}
\toprule
\headrow Arm & $\tau_{50}$ & PickScore & HPSv2.1 & HPSv3 & ImageReward & CLIPScore & Aesthetic & Div.\,$\uparrow$ & Dist.\,$\downarrow$ & PickScore, $200 \times 5$ \\
\midrule
\oursrow \mend{} (reference run, $\tau_0 = \hpTauInit$) & 0.225 & 23.88 & 0.304 & 4.00 & 1.15 & 0.269 & 6.30 & 0.208 & 0.484 & 23.81 \\
Same configuration, second launch & 0.225 & 23.89 & 0.303 & 4.07 & 1.14 & 0.270 & 6.32 & 0.202 & 0.486 & 23.83 \\
$\tau_0 = 0.45$ & 0.200 & 23.90 & 0.302 & 3.86 & 1.12 & 0.270 & 6.33 & 0.203 & 0.487 & 23.83 \\
$\tau_0 = 0.9$ & 0.267 & 23.94 & 0.303 & 3.95 & 1.16 & 0.270 & 6.29 & 0.211 & 0.484 & 23.81 \\
\midrule
One candidate ($K = 1$, $\eta = 0.1$) & 0.225 & 23.90 & 0.302 & 3.74 & 1.14 & 0.271 & 6.26 & 0.203 & 0.487 & 23.79 \\
Five candidates ($\eta \in \{0.05, 0.1, 0.2, 0.4, 0.8\}$) & 0.067 & 23.63 & 0.299 & 3.63 & 1.02 & 0.266 & 6.25 & 0.224 & 0.475 & -- \\
\midrule
No EMA (behavior adapter = trained adapter) & 0.225 & 23.91 & 0.306 & 4.17 & 1.13 & 0.273 & 6.30 & 0.213 & 0.485 & -- \\
PickScore$/\hpRewardDiv$ + HPSv2.1, unit weights & 0.150 & 23.85 & 0.345 & 6.53 & 1.25 & 0.276 & 6.26 & 0.177 & 0.495 & -- \\
\bottomrule
\end{tabular}}
\end{table}

\subsection{One-dimensional toy model}\label{app:hero-toy}
The data density of Figure~\ref{fig:toy} is a mixture of three Gaussians with means $2.2$, $0$, $-2.2$, weights $0.22$, $0.43$, $0.35$ and standard deviations $0.34$, $0.17$, $0.20$; paths are quantile curves of the exact 1D rectified flow from $\mathcal{N}(0,1)$. The true reward is a bump of width $0.2$ at each mode, of height $0.85$ for the top mode and $1$ otherwise, and the learned reward is $\hat R = R + 0.45\,\mathrm{softplus}((|x|-2.27)/0.1)$. Panel (b) is $p\,e^{R/\beta}$ with $\beta = 0.05$; panel (c) takes 18 steps $x \gets x + 0.03\,\hat R'(x)$; panel (d) shows the targets $x + d$ of one \mend{} round on 40{,}000 samples with groups of 8, $q = 0.75$, $\eta \in \{0.15, 0.3, 0.6\}$ and $\tau = 0.25$.

After the round the three modes hold 0.218, 0.430 and 0.353 of the mass (0.217, 0.430 and 0.350 before), while the ascent of panel (c) moves 0.127 of the mass beyond $|x| = 3.25$, where the data has none.
\subsection{The toy over repeated rounds}\label{app:toy-rounds}
\begin{figure}[!htbp]
\centering
\includegraphics[width=\linewidth]{figures/v2_appx/fig_toy_rounds.pdf}
\caption{\textbf{The cap delays drift under a wrong reward.} The three-mode toy over repeated rounds with targets realized exactly: off-data mass and retained hard-mode mass. Dashed lines: KL-tilt fixed points.}
\label{fig:toy-rounds}
\end{figure}
For 15 rounds \mend{}'s targets keep every mode's mass and put at most 0.0003 of the mass off the data, while gradient ascent drains the hard mode and moves 16\% of the mass off the data. From round 16 the learned reward, which keeps rising beyond the data, certifies moves off it, and by round 18 \mend{} has passed gradient ascent.

Proposition~\ref{prop:target} certifies gains in the learned reward; when that reward is wrong in a direction the samples can reach, verification cannot detect the error and the cap only postpones it. This is why we report held-out evaluators and diversity over training.
