# Supplementary material for: MEND: RL For Flow Models via Proximal Velocity Matching
Source: arXiv:2610.05954 source file (2026-10-05)
Supplement: Supplementary file 7 [file v2_G_qualitative.tex]

\section{More qualitative results}\label{app:samples}\label{app:qualitative}
Sample prompts and seeds are selected by eye from images rendered with the same prompts and initial noise for every model; no image was edited, and every number in the tables is over the full prompt sets.

\begin{figure}[!h]
\centering
\includegraphics[width=\linewidth]{figures/v2_appx/verdict_filmstrip.pdf}
\caption{\textbf{A certified move and a kept seed.} Two logged seeds of the rollout policy at update 100, each with its three proposals; bars compare capped gain with price and boxes mark the selected target. Across 1{,}200 logged seeds, 33\% were certified, all at the shortest step.}
\label{fig:verdict-filmstrip}
\end{figure}

\begin{figure}[!htbp]
\centering
\begin{minipage}{0.85\linewidth}
\noindent\parbox[b]{0.2500\linewidth}{\centering\scriptsize SD3.5-M\\base}\parbox[b]{0.2500\linewidth}{\centering\scriptsize Flow-GRPO}\parbox[b]{0.2500\linewidth}{\centering\scriptsize DiffusionNFT}\parbox[b]{0.2500\linewidth}{\centering\scriptsize \textbf{\mend{}\\update 100}}\\[1pt]
\includegraphics[width=\linewidth]{figures/qual/qual_main512_row0.jpg}\\[-1pt]
{\scriptsize Seed 0: Surreal commuter, a man wearing a crossbody bag, calmly walking through a doorway cut into a frozen ocean wave, with impossible physics and cinematic light.}\\[3pt]
\includegraphics[width=\linewidth]{figures/qual/qual_main512_row1.jpg}\\[-1pt]
{\scriptsize Seed 0: Water lily opening at dawn, frog on lily pad, dew, glowing pink petals, still pond reflection and soft mist.}\\[3pt]
\includegraphics[width=\linewidth]{figures/qual/qual_main512_row2.jpg}\\[-1pt]
{\scriptsize Seed 1: Ornate sapphire tiara in a dim museum vitrine, blue stones and diamonds sparkling under spotlight with glass reflections.}\\[3pt]
\includegraphics[width=\linewidth]{figures/qual/qual_main512_row3.jpg}\\[-1pt]
{\scriptsize Seed 0: Macro miniature scene: tiny fisherman on a pebble beside a blue-resin ``lake'' spilling from a bottle; whimsical and detailed.}\\[3pt]
\end{minipage}
\caption{\textbf{Paired samples at 512 pixels.} SD3.5-M, Flow-GRPO, DiffusionNFT and \mend{} at update 100, with shared initial noise; prompts from \citet[Figures~11 to~14]{zhou2026opsd}.}
\label{fig:qual-512}\label{fig:cmp-main}
\end{figure}
\begin{figure}[!htbp]
\centering
\begin{minipage}{0.85\linewidth}
\noindent\parbox[b]{0.2000\linewidth}{\centering\scriptsize SD3.5-M\\update 0}\parbox[b]{0.2000\linewidth}{\centering\scriptsize \mend{}\\update 25}\parbox[b]{0.2000\linewidth}{\centering\scriptsize \mend{}\\update 50}\parbox[b]{0.2000\linewidth}{\centering\scriptsize \mend{}\\update 75}\parbox[b]{0.2000\linewidth}{\centering\scriptsize \textbf{\mend{}\\update 100}}\\[1pt]
\includegraphics[width=\linewidth]{figures/qual/qual_progress_main_row0.jpg}\\[-1pt]
{\scriptsize evaluation seed 46}\\[2pt]
\includegraphics[width=\linewidth]{figures/qual/qual_progress_main_row1.jpg}\\[-1pt]
{\scriptsize evaluation seed 43}
\end{minipage}
\caption{\textbf{One prompt along training.} ``A triangular purple flower pot. A purple flower pot in the shape of a triangle.'' at updates 0 to 100 with fixed initial noise along each row; tiles show PickScore.}
\label{fig:progress-main}
\end{figure}
\begin{figure}[p]
\centering
\newcommand{\seedhead}{\noindent\parbox[b]{0.1667\linewidth}{\centering\scriptsize seed 0}\parbox[b]{0.1667\linewidth}{\centering\scriptsize seed 1}\parbox[b]{0.1667\linewidth}{\centering\scriptsize seed 2}\parbox[b]{0.1667\linewidth}{\centering\scriptsize seed 3}\parbox[b]{0.1667\linewidth}{\centering\scriptsize seed 4}\parbox[b]{0.1667\linewidth}{\centering\scriptsize seed 5}\\[1pt]}
\newcommand{\divrow}[2]{{\scriptsize #2}\\[1pt]\includegraphics[width=\linewidth]{figures/qual/#1}\\[2pt]}
\begin{minipage}[b]{0.495\linewidth}
{\scriptsize A photo of a teddy bear made of water.}\\[1pt]
\seedhead
\divrow{candB_diversity_a_g4.5_row0.jpg}{SD3.5-M, guidance 4.5}
\divrow{candB_diversity_a_g4.5_row1.jpg}{Flow-GRPO, guidance 4.5}
\divrow{candB_diversity_a_g4.5_row2.jpg}{DiffusionNFT, guidance 1}
\divrow{candB_diversity_a_g1_row3.jpg}{\mend{}, update 100, guidance 1}
\divrow{candB_diversity_a_g4.5_row3.jpg}{\mend{}, update 100, guidance 4.5}
\end{minipage}\hfill
\begin{minipage}[b]{0.495\linewidth}
{\scriptsize In late afternoon in January in New England, a man stands in the shadow of a maple tree.}\\[1pt]
\seedhead
\divrow{candB_diversity_b_g4.5_row0.jpg}{SD3.5-M, guidance 4.5}
\divrow{candB_diversity_b_g4.5_row1.jpg}{Flow-GRPO, guidance 4.5}
\divrow{candB_diversity_b_g4.5_row2.jpg}{DiffusionNFT, guidance 1}
\divrow{candB_diversity_b_g1_row3.jpg}{\mend{}, update 100, guidance 1}
\divrow{candB_diversity_b_g4.5_row3.jpg}{\mend{}, update 100, guidance 4.5}
\end{minipage}
\caption{\textbf{Six seeds of two prompts.} Columns share initial noise across methods. Compositions stay similar while prompt fidelity mostly improves.}
\label{fig:diversity}\label{fig:div-main}
\end{figure}
\begin{figure}[!htbp]
\centering
\includegraphics[width=0.9\linewidth]{figures/v2_appx/hires_mosaic.jpg}
\caption{\textbf{\mend{} at 1024 pixels.} Curated tiles from the gallery prompts at native aspect ratios, without upscaling; the pocket-watch tile carries a $2\times$ crop inset.}
\label{fig:hires-mosaic}
\end{figure}
\begin{figure}[p]
\centering
\includegraphics[width=\linewidth,height=0.84\textheight,keepaspectratio]{figures/v2_appx/gallery_1.jpg}
\caption{\textbf{Uncurated gallery sheet.} Seed 0 and shared initial noise for the base at two settings, Flow-GRPO, DiffusionNFT and \mend{} at update 100, with no quality selection.}
\label{fig:hires-uncurated-1}
\end{figure}

\begin{figure}[!htbp]
\centering
\includegraphics[width=\linewidth]{figures/v2/fig_cmp_more.pdf}
\caption{\textbf{More comparison rows.} Same layout as Figure~\ref{fig:cmp}, with PickScore on each tile.}
\label{fig:cmp-more}
\end{figure}

\begin{figure}[!htbp]
\centering
\includegraphics[width=\linewidth]{figures/v2/fig_qual_more.pdf}
\caption{\textbf{More base-to-\mend{} pairs.} Matched prompts and initial noise, extending Figure~\ref{fig:qual}.}
\label{fig:qual-more}
\end{figure}

\paragraph{Prompts of Figures~\ref{fig:hero} to~\ref{fig:cmp2}, \ref{fig:progress-main}, \ref{fig:cmp-more} and~\ref{fig:qual-more}.}
\input{figures/v2/prompts_v2}
