# Supplementary material for: MEND: RL For Flow Models via Proximal Velocity Matching
Source: arXiv:2610.05954 source file (2026-10-05)
Supplement: Supplementary file 8 [file v2_I_related.tex]

\section{Extended related work}\label{app:related}
Flow-GRPO, DanceGRPO, DiffusionNFT and AWM \citep{liu2025flowgrpo,xue2025dancegrpo,zheng2025nft,xue2025awm} reweight the model's own samples and, with a KL penalty of weight $\beta$, target the tilt $\pi_\beta \propto \pi\, e^{R/\beta}$; ReFL, DRaFT and AlignProp \citep{xu2023imagereward,clark2024draft,prabhudesai2023alignprop} move every sample along $\nabla R$ by an amount set by the learning rate. Few of these papers report diversity: FDFO \citep{mcallister2026fdfo}, ReNFT \citep{bao2026renft} and Adjoint Matching \citep{domingo2025adjoint} use DreamSim, and ORW-CFM-W2 \citep{fan2025orwcfm} and DMDR \citep{jiang2025dmdr} use CLIP-embedding and LPIPS distances. Selection methods keep the best of $N$ samples \citep{dong2023raft}, fit samples found by a test-time search \citep{lee2025dav}, accept or reject at an intermediate noise level \citep{anil2026pgraft} or rank fresh candidates \citep{jiang2026drpo}; inference-time guidance \citep{bansal2023universal,chung2023dps,he2024mpgd,meng2022sdedit} applies the reward gradient to the sampler instead of to training targets.
