# Supplementary material for: MEND: RL For Flow Models via Proximal Velocity Matching
Source: arXiv:2610.05954 source file (2026-10-05)
Supplement: Supplementary file 9 [file v2_appendix.tex]

\renewcommand{\floatpagefraction}{0.7}
\renewcommand{\bottomfraction}{0.9}
\setcounter{topnumber}{3}
\setcounter{bottomnumber}{3}
\setcounter{totalnumber}{5}
\makeatletter
\newcommand{\appxFloatBarrier}{\par
  \ifx\@deferlist\@empty\else
    \newpage
    \ifx\@deferlist\@empty\else\clearpage\fi
  \fi}
\makeatother
\makeatletter
\addtocontents{toc}{\protect\setcounter{tocdepth}{2}}
{\centering\large\sc Appendix\par}
\vspace{6pt}
{\noindent\normalsize\bf Contents\par}
\vspace{2pt}
{\small\@starttoc{toc}}
\makeatother
\vspace{10pt}
\input{appendix/v2_A_notation}
\input{appendix/v2_B_settings}
\appxFloatBarrier
\input{appendix/v2_C_proofs}
\input{appendix/v2_D_results}
\input{appendix/v2_E_dynamics}
\input{appendix/v2_F_ablations}
\input{appendix/v2_G_qualitative}
\input{appendix/v2_I_related}
