# Supplementary material for: MEND: RL For Flow Models via Proximal Velocity Matching
Source: arXiv:2610.05954 source file (2026-10-05)
Supplement: Supplementary file 10 [file v2_ci_macros.tex]

\setres{appxci.base45.pick.lo}{22.15}
\setres{appxci.base45.pick.hi}{22.54}
\setres{appxci.base45.hps2.lo}{0.274}
\setres{appxci.base45.hps2.hi}{0.286}
\setres{appxci.base45.hps3.lo}{2.13}
\setres{appxci.base45.hps3.hi}{3.27}
\setres{appxci.base45.ir.lo}{0.72}
\setres{appxci.base45.ir.hi}{0.95}
\setres{appxci.base45.clip.lo}{0.277}
\setres{appxci.base45.clip.hi}{0.290}
\setres{appxci.base45.aes.lo}{5.31}
\setres{appxci.base45.aes.hi}{5.47}
\setres{appxci.base45.div.lo}{0.307}
\setres{appxci.base45.div.hi}{0.344}
\setres{appxci.base45.dist.note}{0 (n/a)}
\setres{appxci.fg.pick.lo}{23.29}
\setres{appxci.fg.pick.hi}{23.73}
\setres{appxci.fg.hps2.lo}{0.310}
\setres{appxci.fg.hps2.hi}{0.321}
\setres{appxci.fg.hps3.lo}{6.63}
\setres{appxci.fg.hps3.hi}{7.42}
\setres{appxci.fg.ir.lo}{1.17}
\setres{appxci.fg.ir.hi}{1.36}
\setres{appxci.fg.clip.lo}{0.273}
\setres{appxci.fg.clip.hi}{0.286}
\setres{appxci.fg.aes.lo}{5.82}
\setres{appxci.fg.aes.hi}{5.97}
\setres{appxci.fg.div.lo}{0.189}
\setres{appxci.fg.div.hi}{0.216}
\setres{appxci.fg.dist.lo}{0.298}
\setres{appxci.fg.dist.hi}{0.329}
\setres{appxci.nft.pick.lo}{23.61}
\setres{appxci.nft.pick.hi}{24.02}
\setres{appxci.nft.hps2.lo}{0.326}
\setres{appxci.nft.hps2.hi}{0.336}
\setres{appxci.nft.hps3.lo}{7.13}
\setres{appxci.nft.hps3.hi}{7.85}
\setres{appxci.nft.ir.lo}{1.41}
\setres{appxci.nft.ir.hi}{1.56}
\setres{appxci.nft.clip.lo}{0.286}
\setres{appxci.nft.clip.hi}{0.298}
\setres{appxci.nft.aes.lo}{5.94}
\setres{appxci.nft.aes.hi}{6.09}
\setres{appxci.nft.div.lo}{0.123}
\setres{appxci.nft.div.hi}{0.137}
\setres{appxci.nft.dist.lo}{0.523}
\setres{appxci.nft.dist.hi}{0.554}
\setres{appxci.cfg45.pick.lo}{23.48}
\setres{appxci.cfg45.pick.hi}{23.91}
\setres{appxci.cfg45.hps2.lo}{0.314}
\setres{appxci.cfg45.hps2.hi}{0.324}
\setres{appxci.cfg45.hps3.lo}{6.71}
\setres{appxci.cfg45.hps3.hi}{7.57}
\setres{appxci.cfg45.ir.lo}{1.23}
\setres{appxci.cfg45.ir.hi}{1.41}
\setres{appxci.cfg45.clip.lo}{0.284}
\setres{appxci.cfg45.clip.hi}{0.297}
\setres{appxci.cfg45.aes.lo}{5.80}
\setres{appxci.cfg45.aes.hi}{5.97}
\setres{appxci.cfg45.div.lo}{0.133}
\setres{appxci.cfg45.div.hi}{0.156}
\setres{appxci.cfg45.dist.lo}{0.297}
\setres{appxci.cfg45.dist.hi}{0.329}
\setres{appxci.base1.pick.lo}{20.44}
\setres{appxci.base1.pick.hi}{20.71}
\setres{appxci.base1.hps2.lo}{0.203}
\setres{appxci.base1.hps2.hi}{0.211}
\setres{appxci.base1.hps3.lo}{$-$6.87}
\setres{appxci.base1.hps3.hi}{$-$5.99}
\setres{appxci.base1.ir.lo}{$-$0.63}
\setres{appxci.base1.ir.hi}{$-$0.42}
\setres{appxci.base1.clip.lo}{0.233}
\setres{appxci.base1.clip.hi}{0.245}
\setres{appxci.base1.aes.lo}{5.09}
\setres{appxci.base1.aes.hi}{5.20}
\setres{appxci.base1.div.lo}{0.564}
\setres{appxci.base1.div.hi}{0.592}
\setres{appxci.base1.dist.note}{0 (n/a)}
\setres{appxci.fin.pick.lo}{23.81}
\setres{appxci.fin.pick.hi}{24.24}
\setres{appxci.fin.hps2.lo}{0.296}
\setres{appxci.fin.hps2.hi}{0.306}
\setres{appxci.fin.hps3.lo}{3.24}
\setres{appxci.fin.hps3.hi}{4.17}
\setres{appxci.fin.ir.lo}{1.03}
\setres{appxci.fin.ir.hi}{1.23}
\setres{appxci.fin.clip.lo}{0.266}
\setres{appxci.fin.clip.hi}{0.279}
\setres{appxci.fin.aes.lo}{6.17}
\setres{appxci.fin.aes.hi}{6.31}
\setres{appxci.fin.div.lo}{0.188}
\setres{appxci.fin.div.hi}{0.218}
\setres{appxci.fin.dist.lo}{0.481}
\setres{appxci.fin.dist.hi}{0.510}
